# Supplementary material for: SAVE: Protagonist Diversification with Structure Agnostic Video Editing
Source: arXiv:2312.02503 source file (2023-12-05)
Supplement: Supplementary file 1 [file X_suppl.tex]

\clearpage
\setcounter{page}{1}
\setcounter{section}{0}

\setcounter{table}{0}
\setcounter{figure}{0}
\maketitlesupplementary

\section{Implementation Details}
\label{sec:suppl_implement}

\noindent
\textbf{Motion Aware Cross-attention Loss.} We provide more details about our cross-attention regularization in Eq.~\ref{eq:attn_loss}. 
Following \cite{wu2022tune,liu2023video}, we utilize the inflated LDM where there are 16 blocks having Transformer layers. 
Empirically, when generating motion masks $M$ we extract the attention scores from spatio-temporal attention in blocks 11--16. We also found that utilizing only a part of spatio-temporal attention scores \ie scores between pixels in each frame and pixels in the first frame, suffices for generating accurate motion masks, helping to accelerate our whole process.

\noindent
\textbf{Experimental details.} Our implementation is based on the publicly available Stable Diffusion v1-4~\footnote{\href{https://huggingface.co/CompVis/stable-diffusion-v1-4}{https://huggingface.co/CompVis/stable-diffusion-v1-4}}. During training, we fine-tune T2I model for 250 steps to pre-register the protagonist word $S_{pro}$ and T2V model for 250 steps to reconstruct the source video by default. During inference, we use DDIM sampler~\cite{song2020denoising} of 50 steps and set classifier-free guidance~\cite{ho2022classifier} to 7.5. We also use decoupled-guidance attention control~\cite{liu2023video} to maintain unchanged parts.

\section{Datasets Details}
\label{sec:suppl_dataset}
Following previous works~\cite{bar2022text2live,wu2022tune,liu2023video}, we collect 12 videos from DAVIS dataset~\cite{perazzi2016benchmark} and YouTube~\cite{liu2023video} with the corresponding source and editing prompts provided by \cite{wu2022tune,liu2023video}. 
We additionally provide editing prompts associated with protagonist changing, where a new protagonist has a largely different body structure from that of the original protagonist. 
Eventually, we composed 48 pairs of videos and text prompts. 
We also evaluate our method on LOVEU-TGVE datasets~\cite{wu2023cvpr} that select 76 videos from DAVIS, YouTube, and other videos having open licenses. 
We adopt the provided editing prompts that are related to an object-change as well as extend the additional editing prompts including challenging cases. 
There is no overlap among the videos in the two datasets.

\section{Additional Analyses}
\label{sec:suppl_analyses}
In this section, we provide additional ablations on other examples along with an analysis of the video editing results as the number of protagonists increases in the video scenes. 

\noindent
\textbf{Additional Ablations.} We conduct the additional ablation studies for other examples, validating the effectiveness of each component in our method. As shown in Fig.~\ref{fig:suppl_ablation}, with temporally expanded text embeddings of the motion word $S_{mot}$, our method effectively learns the motion in the source video. However, the new protagonist (Pikachu) has an awkward appearance with the oddly mixed texture of the original protagonist. Also, the new protagonist follows the motion in the source video in a slightly different way. When applying cross-attention regularization described in Sec.~\ref{subsec:location_bias}, more accurate motion is restored, including eye blinking and head tilting. Meanwhile, the pre-registration strategy described in Sec.~\ref{subsec:pre-registration} disentangles motion from appearance in the source video, where a natural Pikachu appears in the edited video.

\noindent
\textbf{Analysis on Multiple Protagonists.} We also investigate the video editing results across diverse video scenes, especially those featuring multiple protagonists. We found that our method struggles with learning the video scenes involving 5--10 protagonists and wide camera angles. As shown in the bottom row of Fig.~\ref{fig:suppl_multiple}, while editing, our method misses out on several objects among multiple protagonists in the source video and generates incorrect motions. Exploring future endeavors to encompass the movements of multiple protagonists will be an interesting topic.

\section{Additional Qualitative Results}
\label{sec:suppl_results}
In this section, we provide more visualization of video editing results in Fig.~\ref{fig:suppl_qualitative}--\ref{fig:suppl_qualitative_5}. As shown in Fig.~\ref{fig:suppl_qualitative}, other baselines fail to either faithfully reflect an editing prompt or reproduce the motion in the source video. In Fig.~\ref{fig:suppl_qualitative} (left column), all baselines struggle to disentangle the motion from the appearance and render an awkward train that still maintains a similar shape and appearance to the back of the car in the source video. In Fig.~\ref{fig:suppl_qualitative} (right column), TAV~\cite{wu2022tune} and Video-P2P~\cite{liu2023video} generate different movements regarding arms and legs, while FateZero~\cite{qi2023fatezero} adheres closely to the original video. Meanwhile, our method successfully establishes new protagonists (a train and a monkey) accurately following the motion in both videos as $S_{mot}$ adeptly learns the proper motions disentangled from the appearance.

We also compare our method with other baselines using 32-frame videos in Fig.~\ref{fig:suppl_qualitative_2}--\ref{fig:suppl_qualitative_5}. As shown in Fig.~\ref{fig:suppl_qualitative_2}, other baselines struggle to edit a cat in a source video to Pikachu while preserving the motion. TAV~\cite{wu2022tune} and Video-P2P~\cite{liu2023video} render Pikachu in an inconsistent manner, where its ears and arms appear in pairs in some frames. Also, flickered movements exist in the edited videos due to the unstable body structure of Pikachu across frames, as better demonstrated in the attached videos. Meanwhile, FateZero~\cite{qi2023fatezero} generates Pikachu with an intermediate appearance between Pikachu and the cat, unable to disentangle the motion from the appearance. Our method, on the other hand, reproduces the motion from the source video delicately, avoiding collapsed body structure in the newly generated protagonist and preventing close attachment between the new and original protagonists. In Fig.~\ref{fig:suppl_qualitative_3}--\ref{fig:suppl_qualitative_4}, we also supply comparison results using other 32-frame videos, illustrating that our method exhibits a similar pattern \ie achieving both accurate and smooth motion while faithfully adhering to the editing prompt, ensuring a natural appearance.

In Fig.~\ref{fig:suppl_qualitative_5}, we edit both a protagonist (a person) and a prop (a motorcycle) simultaneously using the same source video in Fig.~\ref{fig:suppl_qualitative_4}. Our method effectively changes both the protagonist and the prop, while other baselines face difficulties in editing both objects.

We also supply videos in supplementary materials for careful examination and assessment.

\begin{figure}[t]
\centering
  \includegraphics[width=1\linewidth]{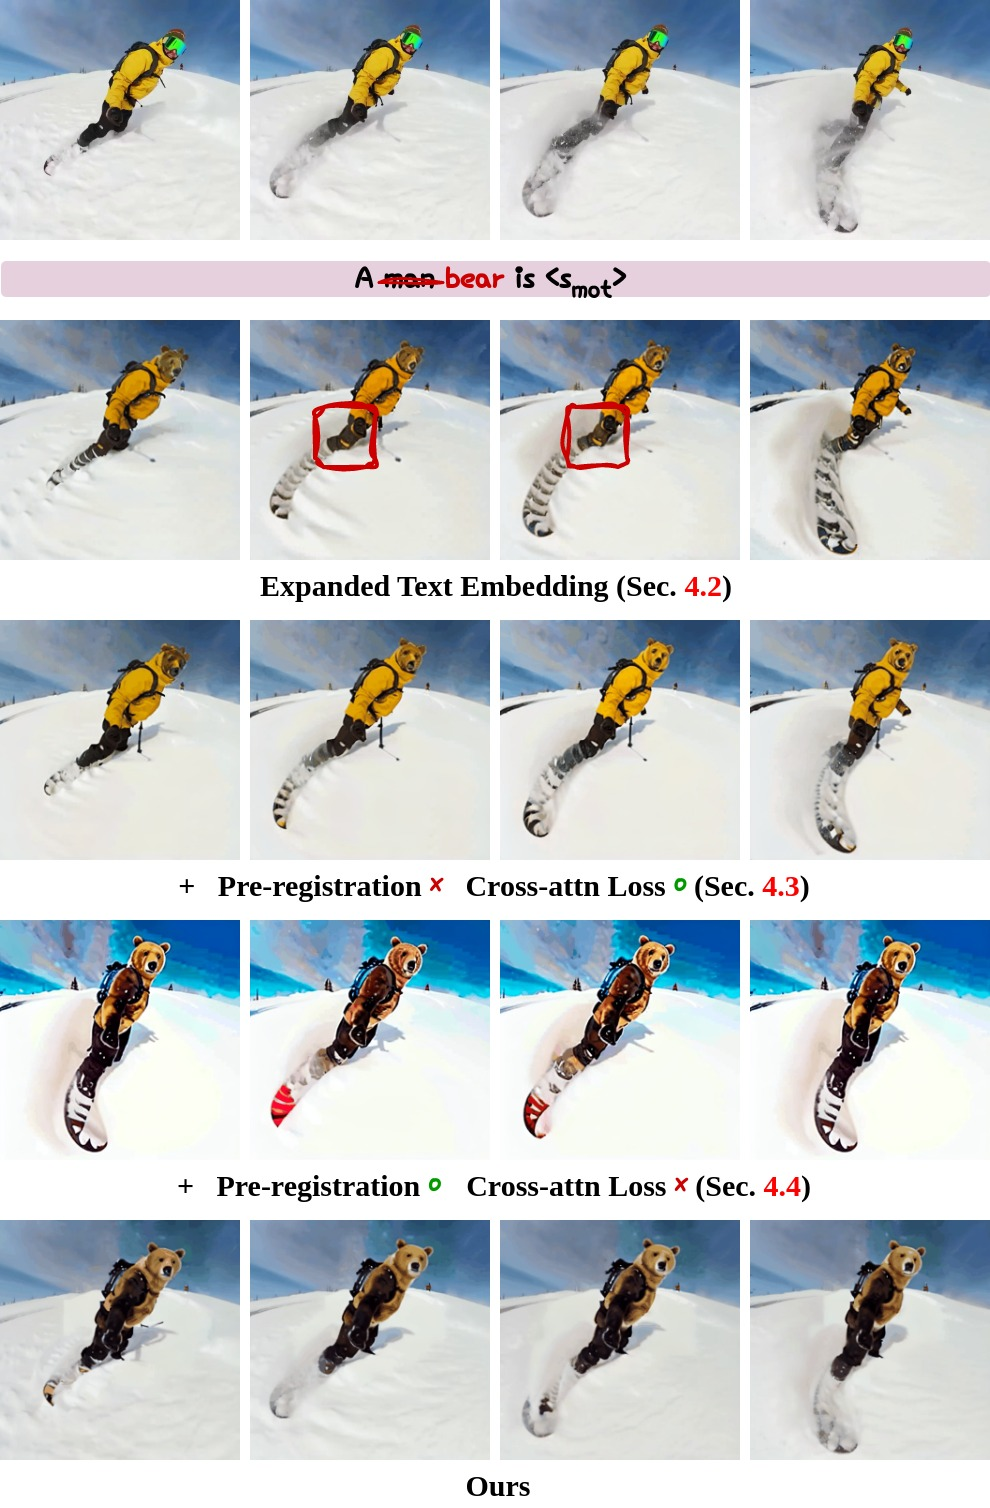}\\
  \caption{\textbf{Ablations on each component.} Employing cross-attention regularization and pre-registration strategy improves accurate motion reproduction and disentanglement, respectively.}
  \label{fig:suppl_ablation}
\end{figure}

% Reference
\newpage
{
    \small
    \bibliographystyle{ieeenat_fullname}
    \bibliography{suppl}
}

% Figures
\begin{figure*}[t]
% \centering
  \includegraphics[width=1\linewidth,right]{figs/Supplement_multiple.png}
  \caption{\textbf{Limitation of our method.} Our method experiences difficulty in handling videos that involve multiple protagonists and wide camera angles. The motion word $S_{mot}$ in those videos should capture various movements in the source video, even when these actions are exhibited within a few pixels throughout the entire scene. An interesting direction for future work involves exploring more complicated and challenging movements and extending $S_{mot}$ to better comprehend and learn these complex movements.}
  \label{fig:suppl_multiple}
\end{figure*}

\begin{figure*}[t]
% \centering
  \includegraphics[width=1.02\linewidth,right]{figs/Supplement_qualitative_1.jpg}
  \caption{\textbf{Additional video editing results comparing our method with other baselines.}}
  \label{fig:suppl_qualitative}
\end{figure*}

\begin{figure*}[t]
% \centering
  \includegraphics[width=1.02\linewidth,right]{figs/Supplement_qualitative_2.jpg}
  \caption{\textbf{Additional video editing results comparing our method with other baselines.}}
  \label{fig:suppl_qualitative_2}
\end{figure*}

\begin{figure*}[t]
% \centering
  \includegraphics[width=1.02\linewidth,right]{figs/Supplement_qualitative_3.jpg}
  \caption{\textbf{Additional video editing results comparing our method with other baselines.}}
  \label{fig:suppl_qualitative_3}
\end{figure*}

\begin{figure*}[t]
% \centering
  \includegraphics[width=1.02\linewidth,right]{figs/Supplement_qualitative_4.jpg}
  \caption{\textbf{Additional video editing results comparing our method with other baselines.}}
  \label{fig:suppl_qualitative_4}
\end{figure*}

\begin{figure*}[t]
% \centering
  \includegraphics[width=1.02\linewidth,right]{figs/Supplement_qualitative_5.jpg}
  \caption{\textbf{Additional results of editing \textit{both} protagonist and another object.}}
  \label{fig:suppl_qualitative_5}
\end{figure*}
